# Supplementary material for: Evaluating the Efficacy of Summarization Evaluation across Languages
Source: arXiv:2106.01478 source file (2021-06-02)
Supplement: Supplementary file 1 [file appendix.pdf]

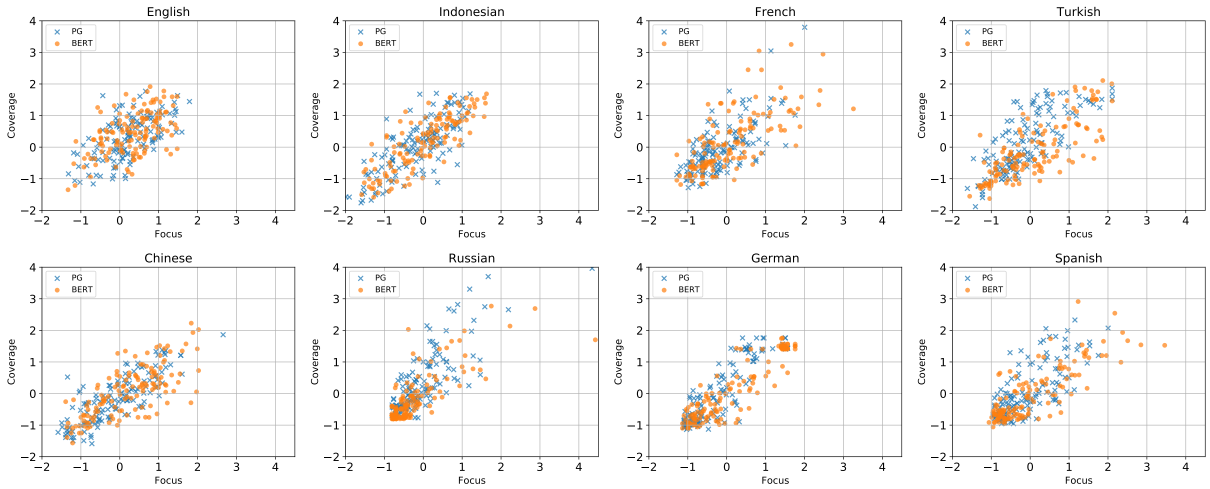


Figure 1: Annotation result (focus vs. coverage) after $z$-score normalization for each of the 8 languages.

| Lang | Model | Recommnded layer | |
|---|---|---|---|
| | | Focus | Coverage |
| EN | `bert-base-uncased` (Devlin et al., 2019) | 1 | 1 |
| ID | `indolem/indobert-base-uncased` (Koto et al., 2020c) | 2 | 2 |
| ZH | `bert-base-chinese` (Devlin et al., 2019) | 8 | 9 |
| FR | `camembert-base` (Martin et al., 2020) | 10 | 9 |
| TR | `dbmdz/bert-base-turkish-uncased` | 12 | 4 |
| RU | `DeepPavlov/rubert-base-cased` (Kuratov and Arkhipov, 2019) | 4 | 12 |
| DE | `bert-base-german-dbmdz-uncased` | 12 | 12 |
| ES | `dccuchile/bert-base-spanish-wwm-uncased` | 4 | 4 |

Table 4: Recommended layers for computing focus and coverage via BERTScore with monolingual model.

| Language | ISO | Data | Data Split | | | Pointer Generator | | | BERT | | |
|---|---|---|---|---|---|---|---|---|---|---|---|
| | | | Train | Dev | Test | R1 | R2 | RL | R1 | R2 | RL |
| English | EN | CNN/DailyMail | 287,226 | 13,368 | 11,490 | 39.53 | 17.28 | 36.38 | 42.13 | 19.60 | 39.18 |
| Indonesian | ID | Liputan6 | 193,883 | 10,972 | 10,792 | 36.10 | 19.19 | 33.56 | 41.08 | 22.85 | 38.01 |
| Chinese | ZH | LCSTS | 2,400,591 | 8,672 | 725 | 32.39 | 19.92 | 29.45 | 38.47 | 25.45 | 35.30 |
| French | FR | MLSUM | 392,902 | 16,059 | 15,828 | 26.50 | 9.49 | 20.30 | 28.52 | 11.73 | 22.51 |
| Turkish | TR | MLSUM | 249,277 | 11,565 | 12,775 | 39.77 | 26.45 | 36.12 | 41.28 | 28.16 | 37.79 |
| Russian | RU | MLSUM | 25,556 | 750 | 757 | 5.39 | 0.60 | 4.62 | 6.01 | 1.02 | 5.75 |
| German | DE | MLSUM | 220,887 | 11,394 | 10,701 | 36.86 | 27.06 | 35.04 | 44.11 | 33.99 | 42.10 |
| Spanish | ES | MLSUM | 266,367 | 10,358 | 13,920 | 25.05 | 7.44 | 19.53 | 26.48 | 9.59 | 21.69 |

Table 5: Details of datasets and ROUGE scores of summarization models used in this study. Except Chinese, we use summaries from the related authors. For MLSUM, we also found slightly different ROUGE-L because we use the original ROUGE package.

| Metrics | POINTER GENERATOR | | | | | | | | | BERT | | | | | | | | |
|---|---|---|---|---|---|---|---|---|---|---|---|---|---|---|---|---|---|---|
| | EN | ID | FR | TR | ZH | RU | DE | ES | Avg | EN | ID | FR | TR | ZH | RU | DE | ES | Avg |
| **Traditional Metrics** | | | | | | | | | | | | | | | | | | |
| ROUGE-1 | 0.61 | **0.68** | 0.54 | 0.82 | 0.81 | 0.52 | 0.85 | 0.50 | 0.67 | 0.62 | 0.70 | 0.73 | **0.81** | 0.78 | 0.59 | 0.89 | 0.54 | 0.71 |
| ROUGE-2 | 0.60 | 0.59 | 0.56 | 0.83 | 0.78 | 0.54 | 0.86 | 0.61 | 0.67 | 0.55 | 0.65 | 0.71 | 0.77 | 0.73 | 0.56 | 0.87 | 0.61 | 0.68 |
| ROUGE-3 | 0.49 | 0.52 | 0.49 | 0.80 | 0.68 | 0.39 | 0.85 | 0.56 | 0.60 | 0.44 | 0.53 | 0.63 | 0.73 | 0.63 | 0.29 | 0.85 | 0.54 | 0.58 |
| ROUGE-L | 0.60 | 0.69 | 0.55 | 0.83 | 0.81 | 0.51 | 0.85 | 0.50 | 0.67 | 0.62 | 0.68 | 0.73 | 0.80 | 0.75 | 0.58 | 0.88 | 0.57 | 0.70 |
| ROUGE-S | 0.61 | 0.62 | 0.48 | 0.79 | 0.70 | 0.55 | 0.83 | 0.50 | 0.64 | 0.59 | 0.67 | 0.64 | 0.76 | 0.69 | 0.59 | 0.86 | 0.51 | 0.66 |
| ROUGE-SU | 0.61 | 0.63 | 0.50 | 0.79 | 0.72 | 0.55 | 0.83 | 0.50 | 0.64 | 0.59 | 0.68 | 0.66 | 0.77 | 0.70 | 0.60 | 0.86 | 0.50 | 0.67 |
| ROUGE-W.12 | 0.60 | 0.67 | 0.56 | 0.83 | 0.81 | 0.52 | 0.86 | 0.49 | 0.67 | 0.61 | 0.66 | 0.72 | 0.79 | 0.74 | 0.55 | 0.88 | 0.57 | 0.69 |
| METEOR | 0.48 | 0.65 | 0.51 | 0.82 | 0.85 | 0.52 | 0.86 | 0.68 | 0.67 | 0.48 | 0.68 | 0.70 | 0.71 | 0.77 | 0.52 | 0.85 | 0.58 | 0.66 |
| BLEU-4 | 0.51 | 0.57 | 0.60 | 0.78 | 0.75 | 0.46 | 0.86 | 0.59 | 0.64 | 0.44 | 0.54 | 0.66 | 0.64 | 0.65 | 0.51 | 0.85 | 0.46 | 0.59 |
| **MoverScore** | | | | | | | | | | | | | | | | | | |
| mono-BERT | 0.61 | 0.67 | 0.63 | **0.88** | 0.80 | **0.65** | **0.90** | 0.60 | 0.72 | 0.56 | 0.63 | 0.74 | 0.77 | 0.73 | 0.61 | 0.89 | 0.58 | 0.69 |
| mBERT (cased) | 0.58 | 0.62 | 0.71 | 0.84 | 0.79 | 0.60 | 0.88 | 0.71 | 0.72 | 0.53 | 0.71 | **0.78** | 0.75 | 0.73 | 0.68 | 0.88 | 0.59 | 0.71 |
| mBERT (uncased) | 0.63 | 0.65 | **0.76** | **0.88** | 0.79 | 0.57 | 0.89 | **0.74** | **0.74** | 0.56 | 0.71 | **0.78** | 0.76 | 0.73 | 0.68 | 0.88 | 0.63 | 0.72 |
| XLM-R (base) | 0.55 | 0.61 | 0.60 | 0.86 | 0.73 | 0.32 | 0.86 | 0.71 | 0.66 | 0.50 | 0.63 | 0.71 | 0.77 | 0.68 | 0.52 | 0.89 | 0.51 | 0.65 |
| XLM-R (large) | 0.52 | 0.57 | 0.60 | 0.84 | 0.62 | 0.30 | 0.87 | 0.63 | 0.62 | 0.49 | 0.58 | 0.69 | 0.76 | 0.52 | 0.42 | 0.87 | 0.46 | 0.60 |
| **BERTScore** | | | | | | | | | | | | | | | | | | |
| mono-BERT | 0.62 | **0.68** | 0.71 | 0.86 | **0.82** | 0.42 | **0.90** | 0.69 | 0.71 | **0.65** | 0.73 | 0.72 | 0.80 | **0.81** | **0.71** | **0.91** | **0.66** | **0.75** |
| mBERT (cased) | 0.61 | 0.67 | 0.64 | 0.84 | 0.77 | 0.54 | 0.89 | 0.69 | 0.71 | 0.58 | **0.74** | 0.76 | **0.81** | 0.77 | **0.71** | **0.91** | 0.54 | 0.73 |
| mBERT (uncased) | **0.64** | **0.68** | 0.67 | 0.86 | 0.79 | 0.48 | 0.89 | 0.70 | 0.72 | 0.63 | 0.72 | 0.73 | **0.81** | 0.77 | 0.69 | 0.90 | 0.57 | 0.73 |
| XLM-R (base) | 0.62 | 0.65 | 0.59 | 0.86 | 0.80 | 0.39 | 0.87 | 0.63 | 0.68 | 0.61 | 0.64 | 0.69 | **0.81** | 0.78 | 0.64 | 0.90 | 0.56 | 0.70 |
| XLM-R (large) | **0.64** | 0.65 | 0.64 | 0.87 | 0.80 | 0.35 | 0.88 | 0.67 | 0.69 | 0.64 | 0.66 | 0.69 | 0.80 | 0.77 | 0.66 | 0.90 | 0.57 | 0.71 |

Table 6: Pearson correlation between automatic metrics and human judgments for **focus** aspect. We compute the precision for ROUGE and BERTScore. All metric is computed by using default configuration of the original implementation.

| Metrics | POINTER GENERATOR | | | | | | | | | BERT | | | | | | | | |
|---|---|---|---|---|---|---|---|---|---|---|---|---|---|---|---|---|---|---|
| | EN | ID | FR | TR | ZH | RU | DE | ES | Avg | EN | ID | FR | TR | ZH | RU | DE | ES | Avg |
| **Traditional Metrics** | | | | | | | | | | | | | | | | | | |
| ROUGE-1 | 0.59 | 0.73 | 0.66 | 0.79 | **0.82** | 0.52 | 0.90 | 0.67 | 0.71 | 0.64 | 0.71 | 0.70 | 0.86 | 0.76 | 0.57 | 0.89 | 0.70 | 0.73 |
| ROUGE-2 | 0.55 | 0.65 | 0.68 | 0.76 | 0.78 | 0.63 | 0.89 | 0.64 | 0.70 | 0.57 | 0.66 | 0.72 | 0.83 | 0.72 | 0.52 | 0.90 | 0.73 | 0.71 |
| ROUGE-3 | 0.49 | 0.59 | 0.58 | 0.69 | 0.68 | 0.50 | 0.88 | 0.57 | 0.62 | 0.45 | 0.55 | 0.66 | 0.79 | 0.63 | 0.41 | 0.89 | 0.64 | 0.63 |
| ROUGE-L | 0.58 | 0.74 | 0.64 | 0.79 | 0.82 | 0.54 | 0.90 | 0.66 | 0.71 | 0.64 | 0.70 | 0.71 | 0.86 | 0.77 | 0.56 | 0.90 | 0.72 | 0.73 |
| ROUGE-S | 0.60 | 0.69 | 0.63 | 0.74 | 0.77 | 0.52 | 0.89 | 0.66 | 0.69 | 0.59 | 0.69 | 0.69 | 0.81 | 0.70 | 0.51 | 0.89 | 0.71 | 0.70 |
| ROUGE-SU | 0.60 | 0.70 | 0.64 | 0.75 | 0.79 | 0.52 | 0.89 | 0.67 | 0.69 | 0.60 | 0.69 | 0.70 | 0.82 | 0.71 | 0.57 | 0.89 | 0.71 | 0.71 |
| ROUGE-W.12 | 0.53 | 0.71 | 0.64 | 0.77 | 0.81 | 0.55 | 0.90 | 0.65 | 0.69 | 0.65 | 0.68 | 0.69 | 0.85 | 0.75 | 0.56 | 0.90 | 0.68 | 0.72 |
| METEOR | 0.60 | 0.72 | 0.65 | 0.77 | 0.81 | 0.55 | 0.89 | 0.63 | 0.70 | 0.66 | 0.69 | 0.69 | 0.83 | 0.75 | 0.59 | 0.89 | 0.75 | 0.73 |
| BLEU-4 | 0.48 | 0.61 | 0.63 | 0.61 | 0.70 | 0.49 | 0.84 | 0.50 | 0.61 | 0.49 | 0.56 | 0.59 | 0.75 | 0.67 | 0.54 | 0.87 | 0.59 | 0.63 |
| **MoverScore** | | | | | | | | | | | | | | | | | | |
| mono-BERT | 0.58 | 0.65 | 0.63 | 0.73 | 0.79 | 0.68 | 0.86 | 0.55 | 0.68 | 0.60 | 0.60 | 0.69 | 0.86 | 0.75 | 0.66 | 0.91 | 0.68 | 0.72 |
| mBERT (cased) | 0.54 | 0.67 | 0.68 | 0.71 | 0.77 | 0.60 | 0.82 | 0.63 | 0.68 | 0.52 | 0.71 | 0.75 | 0.82 | 0.73 | 0.63 | 0.89 | 0.74 | 0.72 |
| mBERT (uncased) | 0.58 | 0.68 | 0.74 | 0.72 | 0.76 | 0.58 | 0.84 | 0.64 | 0.69 | 0.59 | 0.70 | 0.76 | 0.85 | 0.73 | 0.65 | 0.90 | 0.76 | 0.74 |
| XLM-R (base) | 0.56 | 0.61 | 0.52 | 0.68 | 0.71 | 0.31 | 0.82 | 0.62 | 0.60 | 0.57 | 0.64 | 0.68 | 0.83 | 0.65 | 0.52 | 0.90 | 0.68 | 0.68 |
| XLM-R (large) | 0.51 | 0.62 | 0.50 | 0.66 | 0.59 | 0.31 | 0.82 | 0.49 | 0.56 | 0.56 | 0.61 | 0.63 | 0.82 | 0.56 | 0.48 | 0.88 | 0.63 | 0.65 |
| **BERTScore** | | | | | | | | | | | | | | | | | | |
| mono-BERT | 0.64 | 0.74 | **0.76** | **0.87** | 0.81 | **0.72** | **0.92** | **0.73** | **0.78** | **0.68** | **0.74** | **0.78** | **0.89** | 0.78 | 0.63 | **0.92** | **0.78** | **0.77** |
| mBERT (cased) | **0.67** | **0.75** | 0.67 | 0.85 | **0.82** | 0.70 | 0.91 | 0.72 | 0.76 | **0.68** | 0.71 | 0.74 | 0.89 | 0.76 | **0.69** | 0.90 | 0.72 | 0.76 |
| mBERT (uncased) | 0.64 | **0.75** | 0.70 | 0.85 | 0.81 | 0.67 | 0.91 | 0.71 | 0.76 | 0.64 | 0.73 | 0.76 | 0.89 | 0.77 | 0.68 | 0.90 | 0.73 | 0.76 |
| XLM-R (base) | 0.66 | 0.72 | 0.68 | 0.84 | 0.77 | 0.63 | 0.91 | 0.70 | 0.74 | 0.64 | 0.70 | 0.67 | 0.88 | 0.69 | 0.67 | 0.89 | 0.71 | 0.73 |
| XLM-R (large) | 0.66 | 0.70 | 0.68 | 0.84 | 0.77 | 0.59 | 0.91 | 0.70 | 0.73 | 0.66 | 0.69 | 0.70 | 0.88 | 0.70 | **0.69** | 0.90 | 0.72 | 0.74 |

Table 7: Pearson correlation between automatic metrics and human judgments for **coverage** aspect. We compute the recall for ROUGE and BERTScore. All metric is computed by using default configuration of the original implementation.

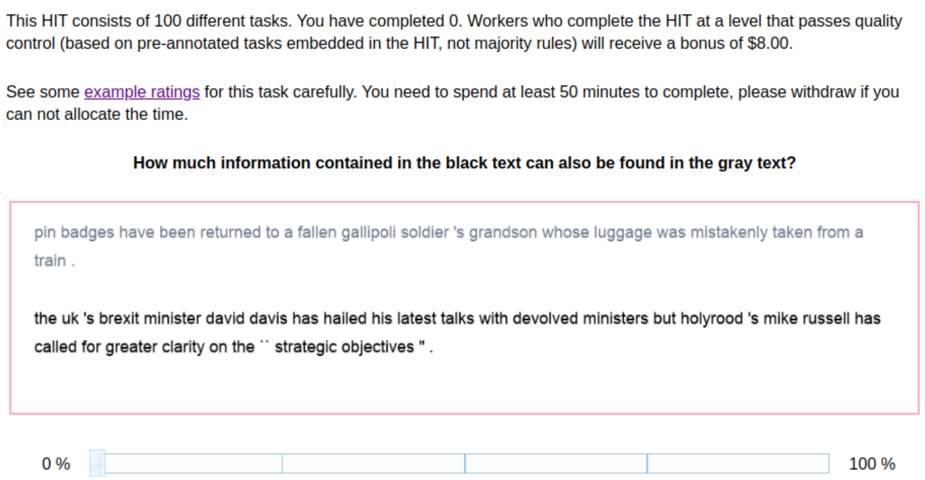


Figure 2: MTurk annotation interface for **English**.

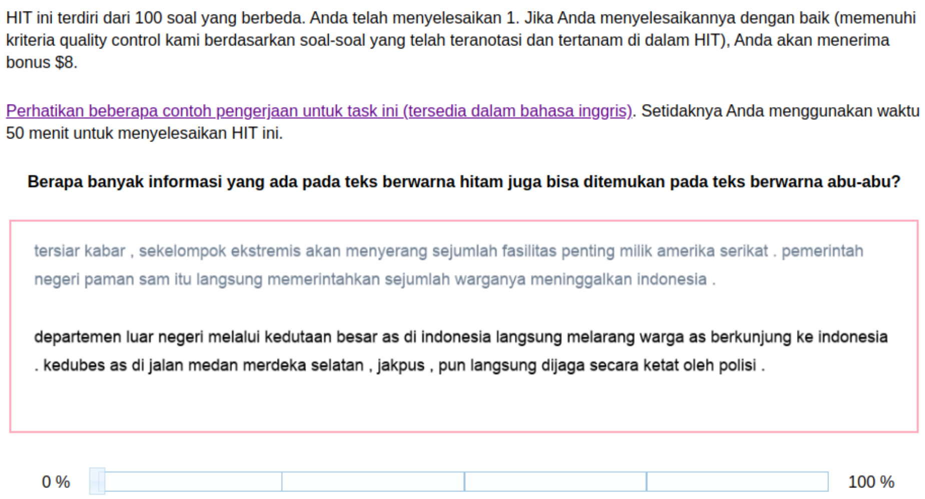


Figure 3: MTurk annotation interface for **Indonesian**.

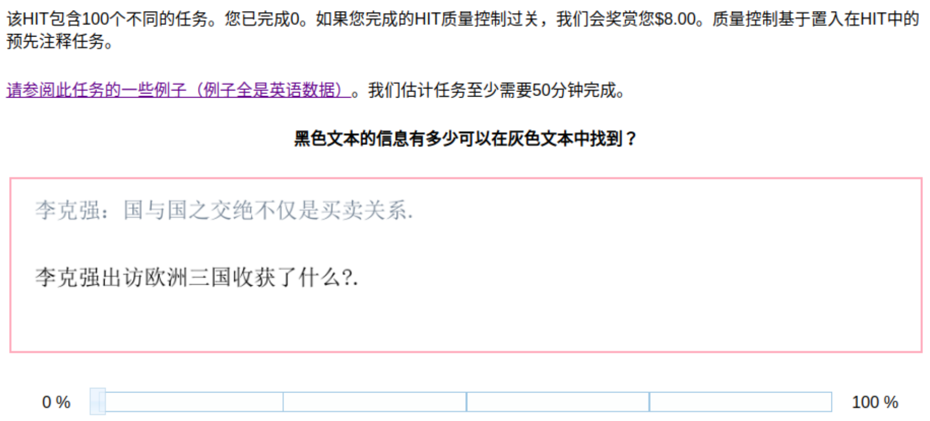


Figure 4: MTurk annotation interface for **Chinese**.

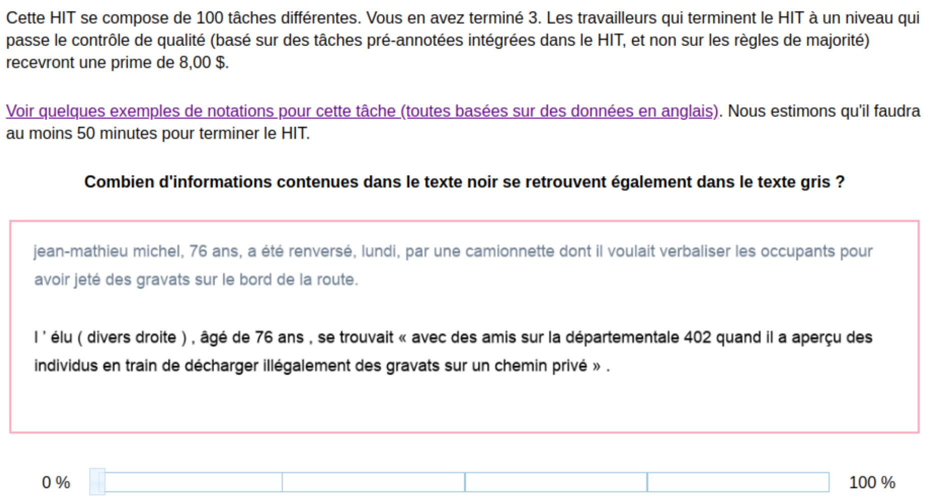


Figure 5: MTurk annotation interface for **French**.

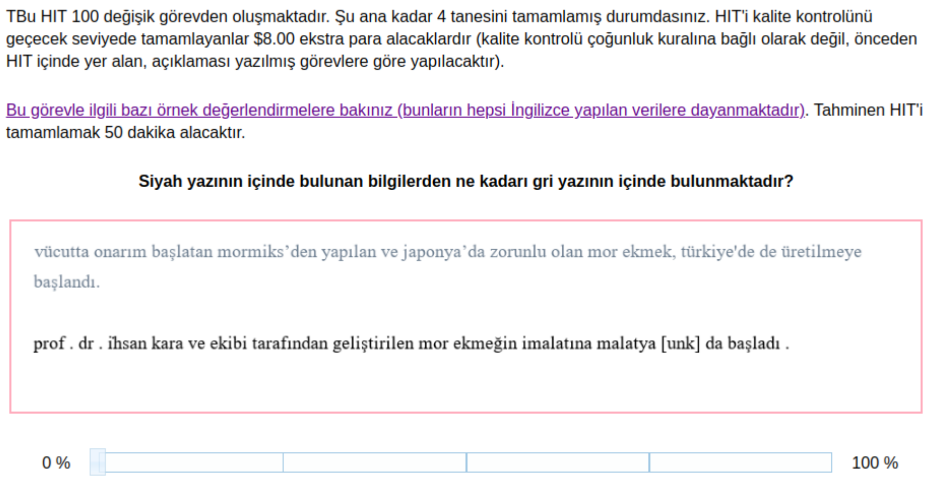


Figure 6: MTurk annotation interface for **Turkish**.

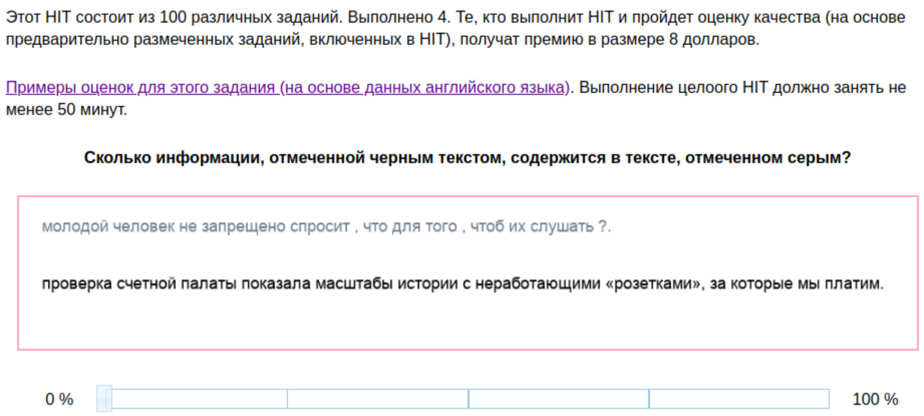


Figure 7: MTurk annotation interface for **Russian**.

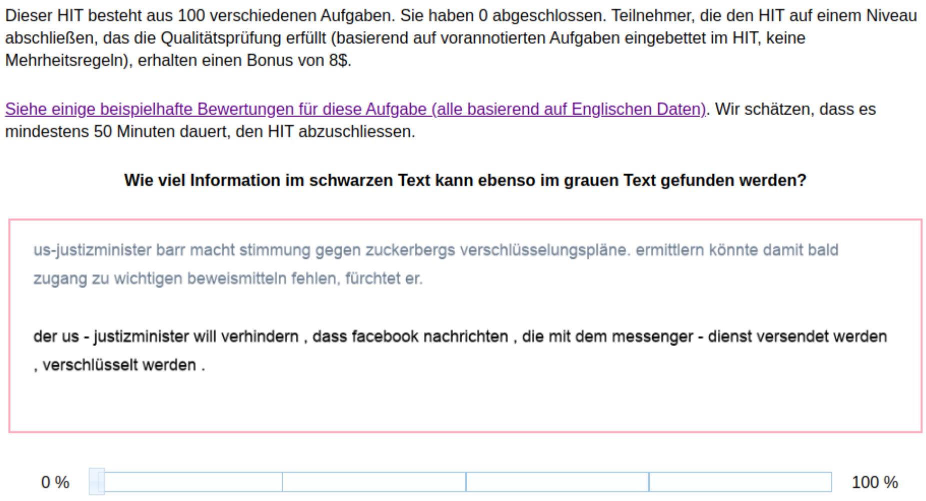


Figure 8: MTurk annotation interface for **German**.

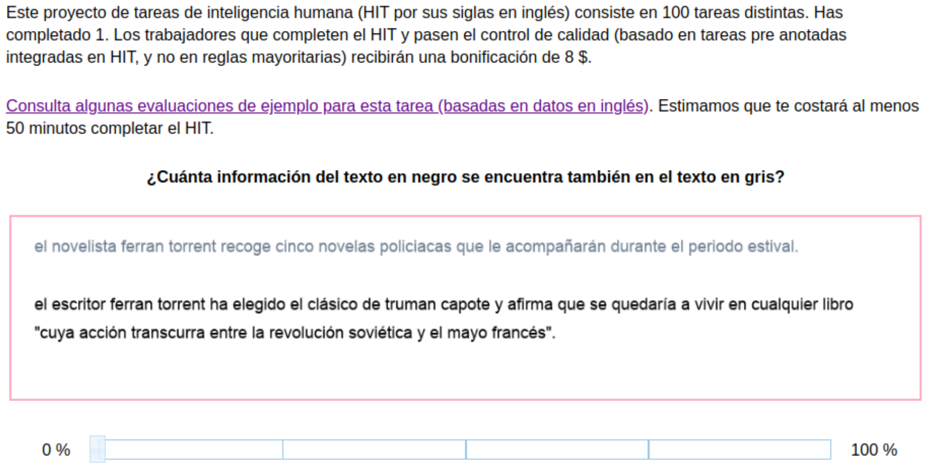


Figure 9: MTurk annotation interface for **Spanish**.
